# Supplementary material for: CED: Color Event Camera Dataset
Source: arXiv:1904.10772 source file (2019-04-24)
Supplement: Supplementary file 1 [file 08_appendix.tex]

\section{Appendix}
\label{sec:appendix}

Here we list the parameters used for each reconstruction method.

\textbf{Manifold Regularisation (MR).}

\textbf{High-pass Filter (HF).}

\textbf{E2VID Neural Network (E2VID).}
